# Supplementary material for: PFLOTRAN-SIP: A PFLOTRAN Module for Simulating Spectral-Induced Polarization of Electrical Impedance Data
Source: arXiv:1909.02125 source file (2020-07-15)
Supplement: Supplementary file 1 [file S8_Appendix.tex]

%===========================================================;
%  Subsection: Main contributions and outline of the paper  ;
%===========================================================;
\subsection{Main contributions and outline of the paper}
\label{SubSec:S1_Main_Contributions}
In this work, we built a coupled framework \texttt{PFLOTRAN-SIP} to simulate flow, solute transport, and SIP processes for a large-scale system.
This framework adds to the recently developed \texttt{PFLOTRAN-E4D} code and takes advantage of the \texttt{PFLORAN-E4D} massively parallel capabilities. 
The paper is organized as follows:~Sec.~\ref{Sec:S1_Intro} discusses the limitations of ERT along with the advantages of the SIP method. 
The importance of coupling between fluid flow, reactive-transport, and SIP process models is discussed.
Discussion on the state-of-the-art simulators are also provided.
Sec.~\ref{Sec:S2_coupling} introduces the \texttt{PFLOTRAN-SIP} framework.
A methodology for coupling \texttt{PFLOTRAN} and \texttt{E4D} simulators is described.
Process models related to SIP, fluid flow, and solute transport in \texttt{PFLOTRAN} and \texttt{E4D} simulators are presented.
% The Archie's model is used as a petrophysical transformation, which links fluid flow and solute transport state variables to bulk electrical conductivity at near zero frequency.
% The Cole-Cole model is used to account for frequency dependence and contains information on the polarization features.
Also, this section discusses the mesh interpolation to transfer state variables between \texttt{PFLOTRAN} and \texttt{E4D} meshes.
Sec.~\ref{Sec:S3_model_framework} describes a reservoir-scale model setup to perform high-fidelity numerical simulations.
It describes the model domain, related meshes, initial conditions, boundary conditions, and various input parameters related to \texttt{PFLOTRAN-SIP} framework.
Additionally, this section provides details on the inversion procedure for electrical conductivity at different frequencies.
This exercise was performed with the intention of comparing the simulated conductivity/tracer distribution from \texttt{PFLOTRAN-SIP} framework and inverted electrical conductivity from SIP inversion.
Sec.~\ref{Sec:S4_Results} explains simulated electrical potentials for a measurement and compares the true/simulated and estimated conductivities.
Also, it shows that estimated frequency-dependent conductivities from the SIP inversion are consistent with the tracer concentration/simulated conductivity from the \texttt{PFLOTRAN-SIP} framework.
Sec.~\ref{Sec:S5_Discussion} provides a discussion on the numerical results, limitations of the proposed framework, and how geoscientists can use the \texttt{PFLOTRAN-SIP} tool for their applications. 
Finally, conclusions are drawn in Sec.~\ref{Sec:S6_Conclusions}.
